# Supplementary material for: Transparent Neighborhood Approximation for Text Classifier Explanation
Source: arXiv:2411.16251 source file (2024-11-25)
Supplement: Supplementary file 1 [file supplemental.tex]

\onecolumn
% \appendices
\setcounter{page}{1}
\setcounter{table}{0}
\setcounter{figure}{0}
\setcounter{section}{0}

% \numberwithin{table}{section}
% \numberwithin{figure}{section}

\begin{center}
\textbf{\LARGE Supplementary Material} \\
\Large Transparent Neighborhood Approximation for Text Classifier Explanation by Probability-based Editing
\end{center}

\section{Experimental Settings} \label{apx:exp_setup}
% 1.1 software and hardware setup
% 1.2 classifier setup, training procedure

\section{Further Example Explanations} \label{apx:quality}
We provide more samples of explanation in Table~\ref{tab:appendix_quality}.
The two special tokens that appear in the examples are $\langle unk\rangle$ and $\langle num\rangle$.
The first represents words out of vocabulary and the other is the generic token for Arabic numbers in texts.
We also want to state that the typos in the presented texts (e.g., ``poion'' instead of ``portion'' in the third sample explanation for the \textit{amazon LSTM} model) are from the datasets rather than mistakes while formatting the results.

According to the shown examples, the word-level explanations from \pbased{} align well with those by \gbased{}.
Its extrinsic words also demonstrate potential for debugging similarly to \gbased{}.
For example, the generic token $\langle num\rangle$ is reported as contributing to negative sentiment in the first example for the \textit{yelp RF} classifier.
The reason behind this is the imbalanced distribution analogous to the ``sausage'' case mentioned in Section~\ref{sec:qualitative}.
Negative comments may refer to complaints about prices and result in the ten times more frequent appearance of the $\langle num\rangle$ token in the negative class than in the positive. 
Thus, the model considers it an important, but in fact, inappropriate observation for its decisions.

The \mbox{(counter-)}factuals from \gbased{}~offer additional information for understandings targeted decisions. 
These factuals underline the importance of certain ingredients showing the consequence of including/excluding them from input texts. 
\pbased{}~drops the generator and sacrifices the generative capacity for a fully transparent neighborhood construction process.
The trade-off between capacity and transparency considerably undermines the quality of its factuals compared to the other since they frequently involve unrealistic grammatical errors and/or semantic conflicts.
We interpret the mistakes by \mbox{(counter-)}factuals from \pbased{} as a consequence of the rather intuitive prototype edition strategy.
\textit{Unigram} is chosen to represent the in-text context for the edition due to the limited size of the corpus.
It encourages editions regardless of their precision.
A countermeasure for this is the extension of the in-text context, namely selecting a greater \textit{n} for the \textit{n}-gram.
Note that the extension of context must couple with an enlarged corpus. 
Otherwise, the method may fail to find any possible operation for seldom observed word sequences.
Besides, the edition operation is determined greedily over iterations, which harms the quality of generated variants in the long run.
A possible solution is restructuring the generated texts over a certain period for their optimal layouts.
But a higher computational cost is foreseeable for both potential improvements. 

\begin{center}
    % \centering
    \begin{footnotesize}
        \begin{longtable}{p{0.47\textwidth} p{0.48\textwidth}} 
            \caption{Example explanations on different classifiers by \gbased{}, \pbased{}}\\
            \hline
            \rowcolor{Gray}
            \multicolumn{2}{p{.975\textwidth}}{\textbf{Input}: why you shouldn't take reviews seriously \hfill Dataset: \textbf{Amazon}, \textbf{RF} $b(\cdot)$: {\textcolor{red}{0.72}}\Tstrut}
            \\[0.2em] \hline
            \\[-1em] 
            \textbf{Saliency}: \hlRed[0.16]{why} you shouldn't take reviews seriously &
            \textbf{Extrinsic words}: \hlBlue[0.19]{must} \hfill \textbf{\gbased{}}\\
            \textbf{Factuals}: & \textbf{Counterfactuals}: \\
            1) why you shouldn't take reviews seriously seriously & 1) why you shouldn't read this seriously\\
            2) why can't take you reviews seriously? & 2) why must you won't write reviews\\
            3) why can't take this reviews seriously & 3) who think that s take on reviews seriously make\\
            4) why s you shouldn't use reviews seriously & 4) why can't take the good script to seriously\\
            5) why you shouldn't write reviews seriously & 5) why can't you write good reviews
            \\[0.38em] \hline \\[-1em] 
            \textbf{Saliency}: \hlRed[0.15]{why} you shouldn't take reviews seriously &
            \textbf{Extrinsic words}: \hlBlue[0.21]{best} \hlBlue[0.19]{great} \hlBlue[0.13]{love} \hfill \textbf{\pbased{}}\\
            \textbf{Factuals}: & \textbf{Counterfactuals}: \\
            1) shouldn why take the reviews. seriously & 1) shouldn't take reviews! seriously\\
            2) why you shouldn't take a pa of reviews with you seriously & 2) shouldn't why you will take a pa of reviews with you seriously\\
            3) you shouldn't take reviews! why & 3) great reviews but why i shouldn't you really take it that seriously\\
            4) you why read the reviews seriously. shouldn't & 4) take you why this simple shouldn't sound this good reviews seriously\\
            5) why t take reviews! seriously & 5) shouldn't take seriously. one of why the best albums i own reviews!
            \\[0.2em] \hline \multicolumn{2}{c}{} \\[-0.5em] \hline

            \rowcolor{Gray}
            \multicolumn{2}{p{.975\textwidth}}{\textbf{Input}: the longest $\langle num\rangle$ minutes in my life \hfill Dataset: \textbf{Amazon}, \textbf{RF} $b(\cdot)$: {\textcolor{blue}{0.65}}\Tstrut}
            \\[0.2em] \hline
            \\[-1em]
            \textbf{Saliency}: the \hlBlue[0.12]{longest} $\langle num\rangle$ minutes in my \hlBlue[0.09]{life} &
            \textbf{Extrinsic words}: \hlRed[0.35]{worst} \hlRed[0.21]{waste} \hlRed[0.18]{after} \hfill \textbf{\gbased{}}\\
            \textbf{Factuals}: & \textbf{Counterfactuals}: \\
            1) the longest $\langle num\rangle$ minutes of my life back & 1) the longest $\langle num\rangle$ minutes after life in my mouth\\
            2) the longest six minutes in my life! & 2) a waste of $\langle num\rangle$ hours of my life\\
            3) the longest movie i have in my life & 3) the longest generation $\langle num\rangle$ you in in my disappointment\\
            4) the longest $\langle num\rangle$ minutes of my life & 4) the worst comedy of all time in my life\\
            5) the longest $\langle num\rangle$ minutes i in my life & 5) not the $\langle num\rangle$ minutes of your life
            \\[0.2em] \hline
            \\[-1em]
            \textbf{Saliency}: the longest $\langle num\rangle$ minutes in my \hlBlue[0.12]{life} &
            \textbf{Extrinsic words}: \hlRed[0.2]{worst} \hlRed[0.17]{waste} \hlRed[0.13]{after} \hfill \textbf{\pbased{}}\\
            \textbf{Factuals}: & \textbf{Counterfactuals}: \\
            1) the longest $\langle num\rangle$ minutes of my life & 1) this is the longest $\langle num\rangle$ minutes\\
            2) in the longest $\langle num\rangle$ minutes $\langle num\rangle$ life & 2) in a waste of $\langle num\rangle$ minutes of my life\\
            3) in the longest! my $\langle num\rangle$ & 3) in the longest! $\langle num\rangle$\\
            4) my life in $\langle num\rangle$ minutes & 4) in the longest $\langle num\rangle$ minutes of my life i ll never get back\\
            5) the longest! my $\langle num\rangle$ minutes & 5) my life $\langle num\rangle$ stars for the longest $\langle num\rangle$ minutes! 
            \\[0.2em] \hline \multicolumn{2}{c}{} \\[-0.5em] \hline
        
            \rowcolor{Gray}
            \multicolumn{2}{p{.975\textwidth}}{\textbf{Input}: the best movie ever! harry, hermione and ron are amazing \hfill Dataset: \textbf{Amazon}, \textbf{RF} $b(\cdot)$: {\textcolor{blue}{0.86}}\Tstrut}
            \\[0.2em] \hline
            \\[-1em] 
            \textbf{Saliency}: the \hlBlue[0.4]{best} movie ever! harry, hermione and ron are \hlBlue[0.06]{amazing} &
            \textbf{Extrinsic words}: \hlRed[0.31]{worst} \hlRed[0.21]{not} \hlRed[0.12]{boring} \hfill \textbf{\gbased{}}\\
            \textbf{Factuals}: & \textbf{Counterfactuals}: \\
            1) the best movie ever! harry potter $\langle unk\rangle$ and ron, amazing! & 1) the worst movie ever, harry potter and $\langle unk\rangle$ are quite wrong\\
            2) the best movie ever! harry potter and $\langle unk\rangle$ sean is original & 2) the worst movie ever ! harry potter $\langle unk\rangle$ and james $\langle unk\rangle$ is\\
            3) the best movie ever! harry potter and $\langle unk\rangle$ sean are amazing & 3) the worst harry potter movie and harry potter was awful\\
            4) the best movie ever! harry potter $\langle unk\rangle$ and ron is quite amazing & 4) the worst movie ever liked this, and $\langle unk\rangle$ were done.\\
            5) the best movie ever! harry potter and $\langle unk\rangle$ sean james! & 5) the worst robin cook ever $\langle unk\rangle$ and ron ever
            \\[0.2em] \hline
            \\[-1em] 
            \textbf{Saliency}: the \hlBlue[0.31]{best} movie ever! harry, hermione and ron are \hlBlue[0.07]{amazing} &
            \textbf{Extrinsic words}: \hlRed[0.43]{worst} \hlRed[0.12]{bad} \hfill \textbf{\pbased{}}\\
            \textbf{Factuals}: & \textbf{Counterfactuals}: \\
            1) the best harry, hermione the best movie ever. ron & 1) ron are the worst movie ever made... harry really, hermione ever\\
            2) are amazing movie, hermione ever! harry!!!!!!!!! & 2) ron are amazing the best worst movie i have ever! harry\\
            3) ron are. and the movie, ever. & 3) amazing the worst. movie, hermione ever.\\
            4) amazing the best horror movie, hermione the best harry. ron & 4) the best worst. ron movie, hermione ever.\\
            5) are and ron movie, hermione ever & 5) harry is amazing, ron movie ever is beyond bad!
            \\[0.2em] \hline \multicolumn{2}{c}{} \\[-0.5em] \hline
        
            \rowcolor{Gray}
            \multicolumn{2}{p{.975\textwidth}}{\textbf{Input}: don't waste your time or money on this one \hfill Dataset: \textbf{Amazon}, \textbf{LSTM} $b(\cdot)$: {\textcolor{red}{0.93}}\Tstrut}
            \\[0.2em] \hline
            \\[-1em]
            \textbf{Saliency}: don't \hlRed[0.25]{waste} your time or \hlRed[0.2]{money} on this one &
            \textbf{Extrinsic words}: \hlRed[0.22]{skip} \hlRed[0.19]{not} \hlBlue[0.14]{best} \hfill \textbf{\gbased{}}\\
            \textbf{Factuals}: & \textbf{Counterfactuals}: \\
            1) don't waste your time or money on this one on this & 1) don't read any time or $\langle unk\rangle$ on this one!\\
            2) don't waste your time or money for this out & 2) don't last time or time on this album\\
            3) make a waste of your time training on the planet & 3) great book for any time or for money on this\\
            4) don't waste your time or money, don t buy this & 4) don't know your time for your projector and this one\\
            5) i don't waste your time or money on this one & 5) the eagles must have your old people on this one
            \\[0.2em] \hline
            \\[-1em]
            \textbf{Saliency}: don t \hlRed[0.3]{waste} your time or \hlRed[0.18]{money} on this one &
            \textbf{Extrinsic words}: \hlBlue[0.12]{great} \hlBlue[0.1]{best} \hfill \textbf{\pbased{}}\\
            \textbf{Factuals}: & \textbf{Counterfactuals}: \\
            1) waste your money on this one time or don & 1) this one of waste your time money on, or don't, a sequal to a great movie\\
            2) waste your money on this one time or don't & 2) this one of his best one on your time money or two! don\\
            3) waste your time money on this one or don & 3) on this the perfect t waste one of your time or!\\
            4) money this one or on don't waste your time & 4) this on a great value for your time or money don\\
            5) your money on this one time or don't waste & 5) don't waste your time with this one, read a good book.
            \\[0.2em] \hline \multicolumn{2}{c}{} \\[-0.5em] \hline
        
            \rowcolor{Gray}
            \multicolumn{2}{p{.975\textwidth}}{\textbf{Input}: it shouldn't be sold. \hfill Dataset: \textbf{Amazon}, \textbf{LSTM} $b(\cdot)$: {\textcolor{red}{0.95}}\Tstrut}
            \\[0.2em] \hline
            \\[-1em]
            \textbf{Saliency}: it \hlRed[0.23]{shouldn't} be \hlRed[0.16]{sold}. &
            \textbf{Extrinsic words}: \hlRed[0.26]{disappointing} \hlRed[0.22]{not} \hfill \textbf{\gbased{}}\\
            \textbf{Factuals}: & \textbf{Counterfactuals}: \\
            1) it shouldn't be sold out. & 1) a masterpiece that should be not.\\
            2) there shouldn't be sold & 2) it s passable but better now!\\
            3) it shouldn't be used. & 3) there must be $\langle num\rangle$.\\
            4) it shouldn't be meant to. & 4) it might be available for its $\langle unk\rangle$.\\
            5) it shouldn't be sold for. & 5) this book should be available made!
            \\[0.2em] \hline
            \\[-1em]
            \textbf{Saliency}: it \hlRed[0.1]{shouldn't} be \hlRed[0.16]{sold}. &
            \textbf{Extrinsic words}: \hlBlue[0.2]{good} \hlBlue[0.09]{must} \hfill \textbf{\pbased{}}\\
            \textbf{Factuals}: & \textbf{Counterfactuals}: \\
            1) shouldn't it be sold. & 1) shouldn it. must be good...\\
            2) shouldn't sold. it be & 2) sold it d be a great collection if...\\
            3) it shouldn't be sold. & 3) it this terrific book shouldn't be sold a civil war novel\\
            4) it shouldn't be. sold & 4) it has gbv sold out? i shouldn't be... this is a great album.\\
            5) shouldn sold it. be... & 5) shouldn't it is to be, it. s up to me!
            \\[0.2em] \hline \multicolumn{2}{c}{} \\[-0.5em] \hline
        
            \rowcolor{Gray}
            \multicolumn{2}{p{.975\textwidth}}{\textbf{Input}: good small poion homemade icecream \hfill Dataset: \textbf{Amazon}, \textbf{LSTM} $b(\cdot)$: {\textcolor{blue}{0.92}}\Tstrut}
            \\[0.2em] \hline
            \\[-1em]
            \textbf{Saliency}: \hlBlue[0.26]{good} \hlRed[0.15]{small} poion homemade icecream &
            \textbf{Extrinsic words}: \hlRed[0.28]{ruined} \hlRed[0.23]{inadequate} \hlRed[0.22]{not} \hfill \textbf{\gbased{}}\\
            \textbf{Factuals}: & \textbf{Counterfactuals}: \\
            1) good small sized $\langle unk\rangle$ soup & 1) good small piece of dutch\\
            2) good small formula type $\langle unk\rangle$ & 2) good small sized type $\langle unk\rangle$\\
            3) good small sized $\langle unk\rangle$ homemade & 3) good value and ruined by foul $\langle unk\rangle$\\
            4) good small pen type $\langle unk\rangle$ & 4) very small sized ruined $\langle unk\rangle$\\
            5) good bit overwhelming $\langle unk\rangle$ & 5) $\langle unk\rangle$ small sized $\langle unk\rangle$
            \\[0.2em] \hline
            \\[-1em]
            \textbf{Saliency}: \hlBlue[0.31]{good} \hlRed[0.13]{small} poion \hlBlue[0.1]{homemade} icecream &
            \textbf{Extrinsic words}: \hlRed[0.26]{too} \hlRed[0.25]{runs} \hfill \textbf{\pbased{}}\\
            \textbf{Factuals}: & \textbf{Counterfactuals}: \\
            1) good small poion homemade icecream & 1) small poion homemade\\
            2) good small poion homemade & 2) good too small poion homemade\\
            3) good to small poion homemade icecream & 3) good content but small poion i didn't know it was homemade icecream\\
            4) good for small poion homemade & 4) only the small poion homemade\\
            5) good it s a small poion homemade & 5) good way too small poion homemade
            \\[0.2em] \hline \multicolumn{2}{c}{} \\[-0.5em] \hline

            \rowcolor{Gray}
            \multicolumn{2}{p{.975\textwidth}}{\textbf{Input}: it's full of fresh ingredients, light and tasty. \hfill Dataset: \textbf{Yelp}, \textbf{RF} $b(\cdot)$: {\textcolor{blue}{0.88}}\Tstrut}
            \\[0.2em] \hline
            \\[-1em]
            \textbf{Saliency}: it's full of \hlBlue[0.25]{fresh} ingredients, light and \hlBlue[0.15]{tasty}. &
            \textbf{Extrinsic words}: \hlRed[0.48]{not} \hlBlue[0.14]{delicious} \hlBlue[0.14]{wood}
             \hfill \textbf{\gbased{}}\\
            \textbf{Factuals}: & \textbf{Counterfactuals}: \\
            1) it's full of ingredients, light and tasty food. & 1) it's full of ingredients, ingredients and light salad.\\
            2) it's full of ingredients, fresh light and tasty. & 2) it's full of ingredients, just light food.\\
            3) it was full of fresh ingredients, light and tasty. & 3) i ate different variety of ingredients and light salad.\\
            4) it's full of fresh ingredients, light and tasty variety. & 4) it's full of all ingredients and light groups.\\
            5) it's full of ingredients and light on food. & 5) it's full of ingredients, not light and tasty.
            \\[0.2em] \hline
            \\[-1em]
            \textbf{Saliency}: it's full of \hlBlue[0.26]{fresh} ingredients, light \hlBlue[0.18]{and} \hlBlue[0.13]{tasty}. &
            \textbf{Extrinsic words}: \hlRed[0.41]{\textlangle \textit{num}\textrangle} \hlRed[0.12]{was} \hlRed[0.1]{over}
             \hfill \textbf{\pbased{}}\\
            \textbf{Factuals}: & \textbf{Counterfactuals}: \\
            1) full of it was light and fresh ingredients. & 1) light of the ingredients are full!!!.\\
            2) light of our breakfast was tasty tasty tasty and fresh ingredients. & 2) of it tasty fresh, wasn't tasty/fresh enough to have been over \$$\langle num\rangle$.\\
            3) full of fresh tasty. & 3) it was light and ingredients.\\
            4) it and they have a full of ingredients, light,. & 4) light was full, tasty's.\\
            5) light was tasty fresh ingredients. & 5) it $\langle num\rangle$ fresh, and fresh, fresh ingredients.
            \\[0.2em] \hline \multicolumn{2}{c}{} \\[-0.5em] \hline
            
            \rowcolor{Gray}
            \multicolumn{2}{p{.975\textwidth}}{\textbf{Input}: it was super dry and had a weird taste to the entire slice. \hfill Dataset: \textbf{Yelp}, \textbf{RF} $b(\cdot)$: {\textcolor{red}{0.81}}\Tstrut}
            \\[0.2em] \hline
            \\[-1em]
            \textbf{Saliency}: it was super \hlRed[0.15]{dry} and had a weird taste to the entire slice. &
            \textbf{Extrinsic words}: \hlBlue[0.35]{delicious} \hlBlue[0.32]{nice} \hlBlue[0.29]{good}
             \hfill \textbf{\gbased{}}\\
            \textbf{Factuals}: & \textbf{Counterfactuals}: \\
            1) it was super dry and had a weird taste and the whole slice. & 1) it was super dry and had a good taste to the entire slice.\\
            2) it was super dry and had a weird taste of the whole plate. & 2) it was super good and had a weird taste to my half slice.\\
            3) it was super dry and had a weird taste to my half slice. & 3) it was very dry and had a good taste of the whole plate.\\
            4) it was super dry and had a taste flavor to the whole slice. & 4) and it was totally the flavor of the meal.\\
            5) it was super dry and had a weird taste to my whole slice. & 5) it was super dry and had a nice taste of the entire slice.
            \\[0.2em] \hline
            \\[-1em]
            \textbf{Saliency}: it \hlRed[0.15]{was} super \hlRed[0.19]{dry} \hlBlue[0.21]{and} had a \hlRed[0.13]{weird} taste to the entire slice. &
            \textbf{Extrinsic words}: \hlBlue[0.46]{great} \hlBlue[0.28]{delicious} \hlBlue[0.27]{good}
             \hfill \textbf{\pbased{}}\\
            \textbf{Factuals}: & \textbf{Counterfactuals}: \\
            1) slice was the entire people here are super weird and taste. & 1) entire a super weird, taste.\\
            2) i had to the dry and it was a weird. & 2) dry and slice.\\
            3) to it dry food taste a slice & 3) entire slice and had to it was super good.\\
            4) entire it had was a weird, but was n't super dry. & 4) it and had the taste was very weird.\\
            5) and it to the entire taste was dry! & 5) super dry and slice.
            \\[0.2em] \hline \multicolumn{2}{c}{} \\[-0.5em] \hline

            \rowcolor{Gray}
            \multicolumn{2}{p{.975\textwidth}}{\textbf{Input}: the food is excellent and the service is exceptional! \hfill Dataset: \textbf{Yelp}, \textbf{RF} $b(\cdot)$: {\textcolor{blue}{0.96}}\Tstrut}
            \\[0.2em] \hline
            \\[-1em]
            \textbf{Saliency}: the food is \hlBlue[0.24]{excellent} \hlBlue[0.19]{and} the \hlBlue[0.08]{service} is \hlBlue[0.11]{exceptional}! &
            \textbf{Extrinsic words}: \hlRed[0.35]{not} \hlRed[0.17]{horrible} \hlRed[0.16]{awful}
             \hfill \textbf{\gbased{}}\\
            \textbf{Factuals}: & \textbf{Counterfactuals}: \\
            1) the food is excellent and the service is superb! & 1) the food is good, and not service at all.\\
            2) the food is excellent, and the service is phenomenal! & 2) the food is not incredible and the service is mediocre at best.\\
            3) the food is excellent and the service is exceptional at best & 3) the food is satisfying and the bill was exceptional.\\
            4) the food is excellent and the service is at! & 4) the food, oh my, the room was/is fabulous.\\
            5) the food is excellent and the service was exceptional. & 5) the food is horrible and the service is bad!!
            \\[0.2em] \hline            
            \\[-1em]
            \textbf{Saliency}: the food is \hlBlue[0.3]{excellent} \hlBlue[0.17]{and} the service is exceptional! &
            \textbf{Extrinsic words}: \hlRed[0.11]{nothing} \hlRed[0.09]{average}
             \hfill \textbf{\pbased{}}\\
            \textbf{Factuals}: & \textbf{Counterfactuals}: \\
            1) excellent food and the service is exceptional. & 1) is the food service was exceptional!.\\
            2) is the food?! & 2) the $\langle num\rangle$ star is for the appetizer and the server's excellent service.\\
            3) excellent and the exceptional service is. & 3) the service is exceptional.\\
            4) excellent food is average and the service is exceptional. & 4) the food is ok... but the service is exceptional.\\
            5) excellent and is the food exceptional & 5) the food is nothing exceptional!
            \\[0.2em] \hline \multicolumn{2}{c}{} \\[-0.5em] \hline

            \rowcolor{Gray}
            \multicolumn{2}{p{.975\textwidth}}{\textbf{Input}: the cake portion was extremely light and a bit dry. \hfill Dataset: \textbf{Yelp}, \textbf{LSTM} $b(\cdot)$: {\textcolor{blue}{0.7}}\Tstrut}
            \\[0.2em] \hline
            \\[-1em]
            \textbf{Saliency}: the cake portion was extremely \hlBlue[0.33]{light} and a bit \hlRed[0.27]{dry}. &
            \textbf{Extrinsic words}: \hlBlue[0.36]{tasty} \hlBlue[0.3]{awesome} \hlBlue[0.29]{generous}
             \hfill \textbf{\gbased{}}\\
            \textbf{Factuals}: & \textbf{Counterfactuals}: \\
            1) the cake was extremely generous and a light over dry tuna. & 1) the cake was extremely large and a bit over dry.\\
            2) the cake portion is large and heavy to a smooth. & 2) the cake portion was extremely light and a tad dry.\\
            3) the cake itself was extremely light and a bit dry. & 3) the cake portion was extremely large and a bit dry.\\
            4) the cake cake was extremely tasty and a gummy dry. & 4) the cake portion was extremely light and a dry dry.\\
            5) the cake portion was extremely thick and a light dry. & 5) the cake was extremely small and light in a dry.
            \\[0.2em] \hline
            \\[-1em]
            \textbf{Saliency}: the \hlBlue[0.09]{cake} portion was extremely \hlBlue[0.33]{light} and a bit \hlRed[0.46]{dry}. &
            \textbf{Extrinsic words}: \hlBlue[0.22]{best} \hlRed[0.22]{however}
             \hfill \textbf{\pbased{}}\\
            \textbf{Factuals}: & \textbf{Counterfactuals}: \\
            1) the cake was extremely light and a bit dry. & 1) and the cake portion was extremely dry.\\
            2) extremely portion - & 2) light was a bit dry.\\
            3) the portion was bit dry and light, at best cake. & 3) the cake portion was a bit.\\
            4) the cake portion was light. & 4) portion is extremely dry and a light.\\
            5) crust is extremely dry and portion was a light. & 5) light and the cake was bit dry.
            \\[0.2em] \hline \multicolumn{2}{c}{} \\[-0.5em] \hline

            \rowcolor{Gray}
            \multicolumn{2}{p{.975\textwidth}}{\textbf{Input}: it was super dry and had a weird taste to the entire slice. \hfill Dataset: \textbf{Yelp}, \textbf{LSTM} $b(\cdot)$: {\textcolor{red}{1.0}}\Tstrut}
            \\[0.2em] \hline
            \\[-1em]
            \textbf{Saliency}: it was \hlBlue[0.08]{super} \hlRed[0.45]{dry} and had a \hlRed[0.17]{weird} \hlRed[0.17]{taste} to the entire slice. &
            \textbf{Extrinsic words}: \hlBlue[0.4]{great} \hlBlue[0.3]{delicious} \hlRed[0.24]{sour}
             \hfill \textbf{\gbased{}}\\
            \textbf{Factuals}: & \textbf{Counterfactuals}: \\
            1) it was super dry and had a weird taste to the whole slice. & 1) it was super dry and had a sweet flavor to the entire combination.\\
            2) it was super dry and had a weird taste to my half slice. & 2) it was perfectly cooked and had a flavor taste and the whole.\\
            3) it was super dry and had a nice taste of the entire slice. & 3) very dry and had a good flavor to a nice slice of the strip\\
            4) it was perfectly dry and had a flavor taste and the whole. & 4) it was super awesome and had the $\langle unk\rangle$ taste to the half.\\
            5) it was super dry and had a weird taste to the half. & 5) it was so good and had a flavor to the whole dish.
            \\[0.2em] \hline
            \\[-1em]
            \textbf{Saliency}: it was \hlBlue[0.25]{super} \hlRed[0.27]{dry} \hlBlue[0.09]{and} had a \hlRed[0.23]{weird} taste to the entire slice. &
            \textbf{Extrinsic words}: \hlBlue[0.34]{great} \hlBlue[0.33]{fresh} \hlBlue[0.29]{good}
             \hfill \textbf{\pbased{}}\\
            \textbf{Factuals}: & \textbf{Counterfactuals}: \\
            1) super dry it is weird to slice at and delicious to taste. & 1) slice it was the entire super good dry.\\
            2) had the entire way you slice it was weird. & 2) weird and a great taste.\\
            3) to and the taste was a super dry. & 3) entire slice i super loved it had dry.\\
            4) entire a super weird. & 4) slice and it was super fresh taste weird.\\
            5) had to the taste was a slice. & 5) entire and it was super fresh taste weird.
            \\[0.2em] \hline \multicolumn{2}{c}{} \\[-0.5em] \hline

            \rowcolor{Gray}
            \multicolumn{2}{p{.975\textwidth}}{\textbf{Input}: but service was horrible both times. \hfill Dataset: \textbf{Yelp}, \textbf{LSTM} $b(\cdot)$: {\textcolor{red}{1.0}}\Tstrut}
            \\[0.2em] \hline
            \\[-1em]
            \textbf{Saliency}: \hlRed[0.1]{but} service was \hlRed[0.69]{horrible} \hlBlue[0.11]{both} times. &
            \textbf{Extrinsic words}: \hlRed[0.44]{disappointing} \hlRed[0.42]{different} \hlBlue[0.3]{excellent}
             \hfill \textbf{\gbased{}}\\
            \textbf{Factuals}: & \textbf{Counterfactuals}: \\
            1) but the service was horrible times. & 1) but the service was enjoyed each.\\
            2) but service was horrible both times times. & 2) but it was friendly and both times.\\
            3) but service was horrible and both times. & 3) but the service was always friendly times.\\
            4) but service was horrible and times. & 4) but service was truly enjoyed times.\\
            5) but it was horrible both times. & 5) the service was friendly and prompt.
            \\[0.2em] \hline
            
            \\[-1em]
            \textbf{Saliency}: but service was \hlRed[0.65]{horrible} \hlBlue[0.16]{both} times. &
            \textbf{Extrinsic words}: \hlBlue[0.3]{super} \hlBlue[0.23]{great}
             \hfill \textbf{\pbased{}}\\
            \textbf{Factuals}: & \textbf{Counterfactuals}: \\
            1) both times but was horrible service & 1) but horrible service was both times are great!\\
            2) but service was horrible both times! & 2) both times was but service\\
            3) both times was horrible but service & 3) service was horrible but both delicious!\\
            4) service was horrible but both times! & 4) horrible both good food + good service = good times.\\
            5) service but was horrible both times! & 5) both times, great food but super horrible service was!
            \\[0.2em] \hline 
            \label{tab:appendix_quality}
        \end{longtable}
    \end{footnotesize}
\end{center}

\section{Sensitivity to hyperparameters} \label{apx:parameter}
% \subsection{Sensitivity to hyperparameters} \label{sec:parameter}
To study the influence of the hyperparameters on explanation quality, we repeated the quantitative evaluation with different hyperparameter choices for \gbased{}~and \pbased{}.
In \gbased{}, the two hyperparameters dominating the latent space exploration are the interpolation step $s$ and the number of landmarks $k$.
The neighborhood size is another factor in the neighborhood construction process.
But it is excluded from the analysis of hyperparameter sensitivity since the number of generated instances is highly dependent on the other two parameters and does not reach the limitation in most cases.
We picked the interpolation steps from 6 to 14 with an interval of 2 with the landmark set having a size of 20.
For the test on the landmark number, the values vary from 10 to 30 while keeping the interpolation step at 10.
As for \pbased{}, we tested its sensitivity to the choices of the neighborhood size $p$ (the population limitation) and the number of prototypes $k$.
These are the only two parameters that affect the construction process.
Compared to \gbased{}~(demonstrated in Table~\ref{tbl:effectiveness}), the lower time complexity of \pbased{}~allows us to determine the hyperparameter choices on a larger scale to highlight their effects.
For the population limitation, we chose five values that increase exponentially from 100 to 1600 with the prototype quantity set to 80.
Similarly, we also picked a geometric sequence for $k$ while the population sticks to 400.

For \gbased{}, Fig.~\ref{fig:xproaIntpl} shows that the interpolation intervals from the selected range have limited influence on the three Cs.
The reason for the observation is the continuous distribution in the latent space.
The increase in interpolation density only produces more duplicated instances, which are later removed during the neighborhood finalization.
On the other hand, the increasing size of the landmark set slightly improves the completeness and compactness, as visualized in Fig.~\ref{fig:xproaLm}.
The larger landmark set not only affects the initialization of the progressive approximation but also allows the usage of more landmarks during the iterative interpolation, which encourages latent space exploration and highlights the decision boundary.

Similar changes in confidence drop and in AOPC hold for \pbased{}~with the expansion of the prototype set (Fig.~\ref{fig:xprobLm}), which also affects the initialization along with the intermediate prototype selection.
Partly owing to the larger gaps between the hyperparameter choices, the increasing tendencies are more significant.
The changes in completeness suggest that more relevant features are filtered out and involved in manipulations.
And for the two classifiers trained on the yelp dataset, the saturation of confidence drop holds their DpMs back, which aligns with our argument in Section~\ref{sec:quantitative} about having AOPC as another compactness metric.
In contrast to the changing tendency of completeness, the dropping $R^2$ scores suggest that an excessive amount of prototypes can violate the locality constraint.
The expanding prototype set includes additional parts of the decision boundary and finally introduces non-linearity when it reaches far enough. 
But the explanation qualities remain steady even with a badly chosen $k$ ($=160$) because of the neighborhood approximation and the weighted loss function.
The former tightens the neighborhood, and the latter encourages the surrogate to concentrate on the closer samples by assigning them higher weights.
% ----------------------------
Meanwhile, Fig.~\ref{fig:xprobPopu} illustrates that enriching the neighborhood set also lays positive effects on explanation qualities.
According to all listed metrics, the performances improve rapidly with the growing population, especially when the number is low, and the upward trend slows down once $p$ reaches 400.
The observation indicates that explanations become precise when the population is large enough for proper coverage of neighborhoods.
After that, enrichment of neighboring samples would not further promote explanation qualities.
% Three testing cases out of the four obey the preceding description, but with one exception, whose completeness and AOPC experience a decline in the range between 400 and 1600.

\begin{figure*}
    \centering
    \begin{subfigure}[b]{1.\textwidth}
        \centering
        \includegraphics[width=\textwidth]{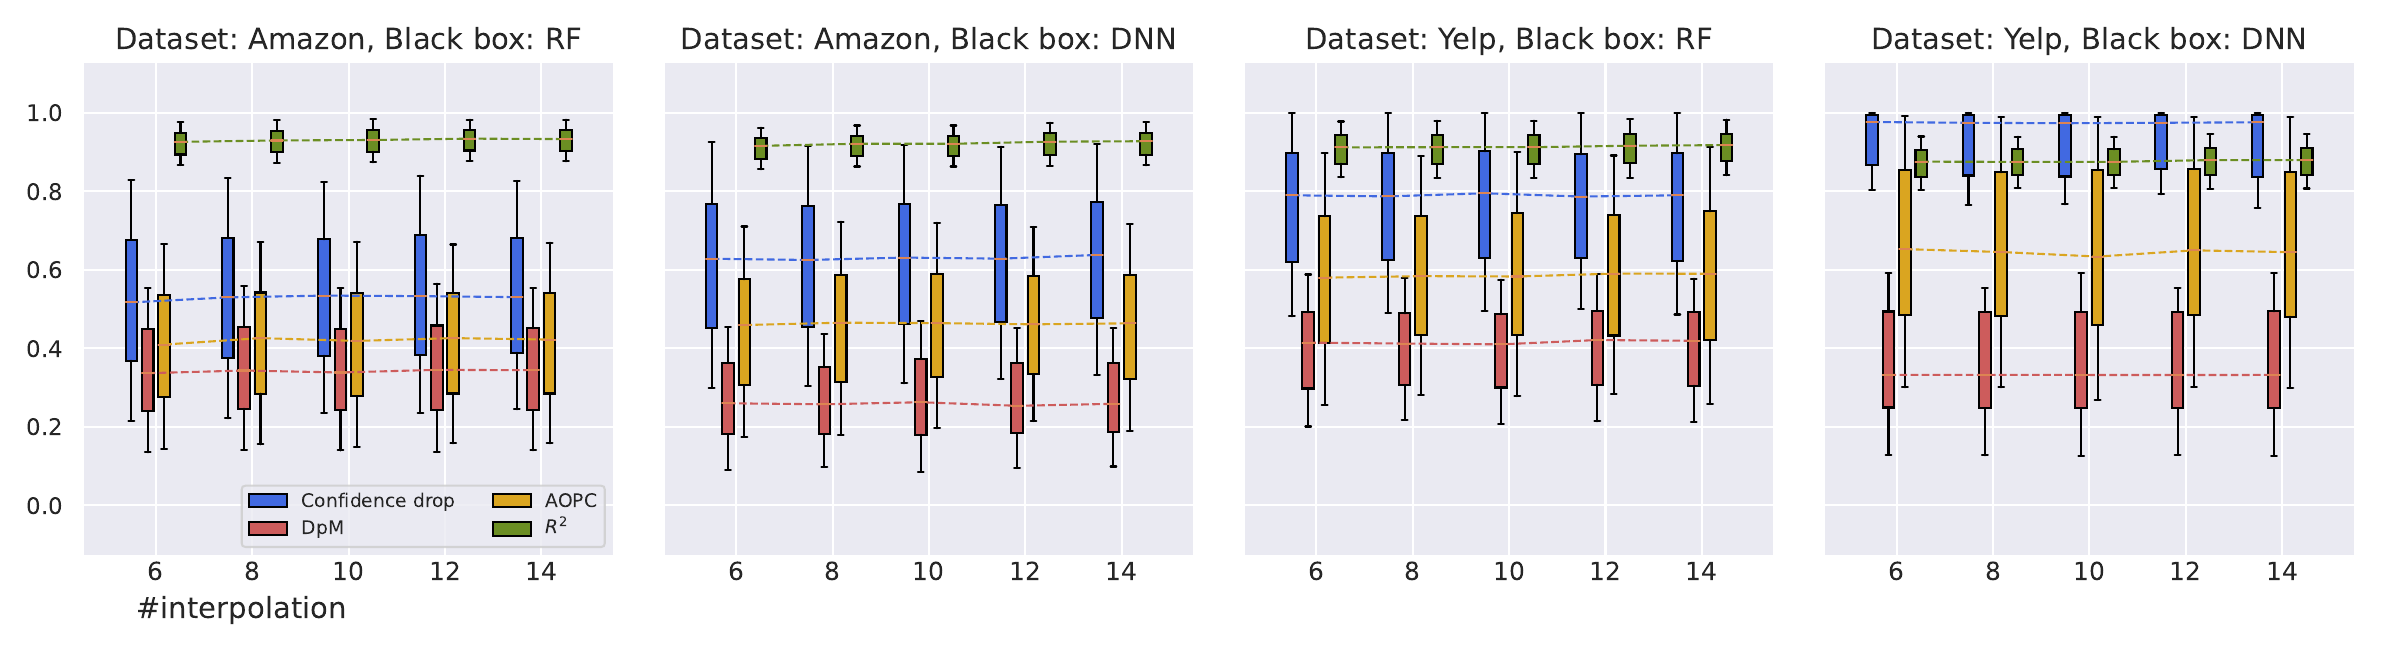}
        \vspace*{-8mm}
        \caption{Sensitivity to the interpolation interval, the number of landmarks is fixed to 20.}
        \label{fig:xproaIntpl}
    \end{subfigure}
    \vspace*{3mm}
    \begin{subfigure}[b]{1.\textwidth}
        \centering
        \includegraphics[width=\textwidth]{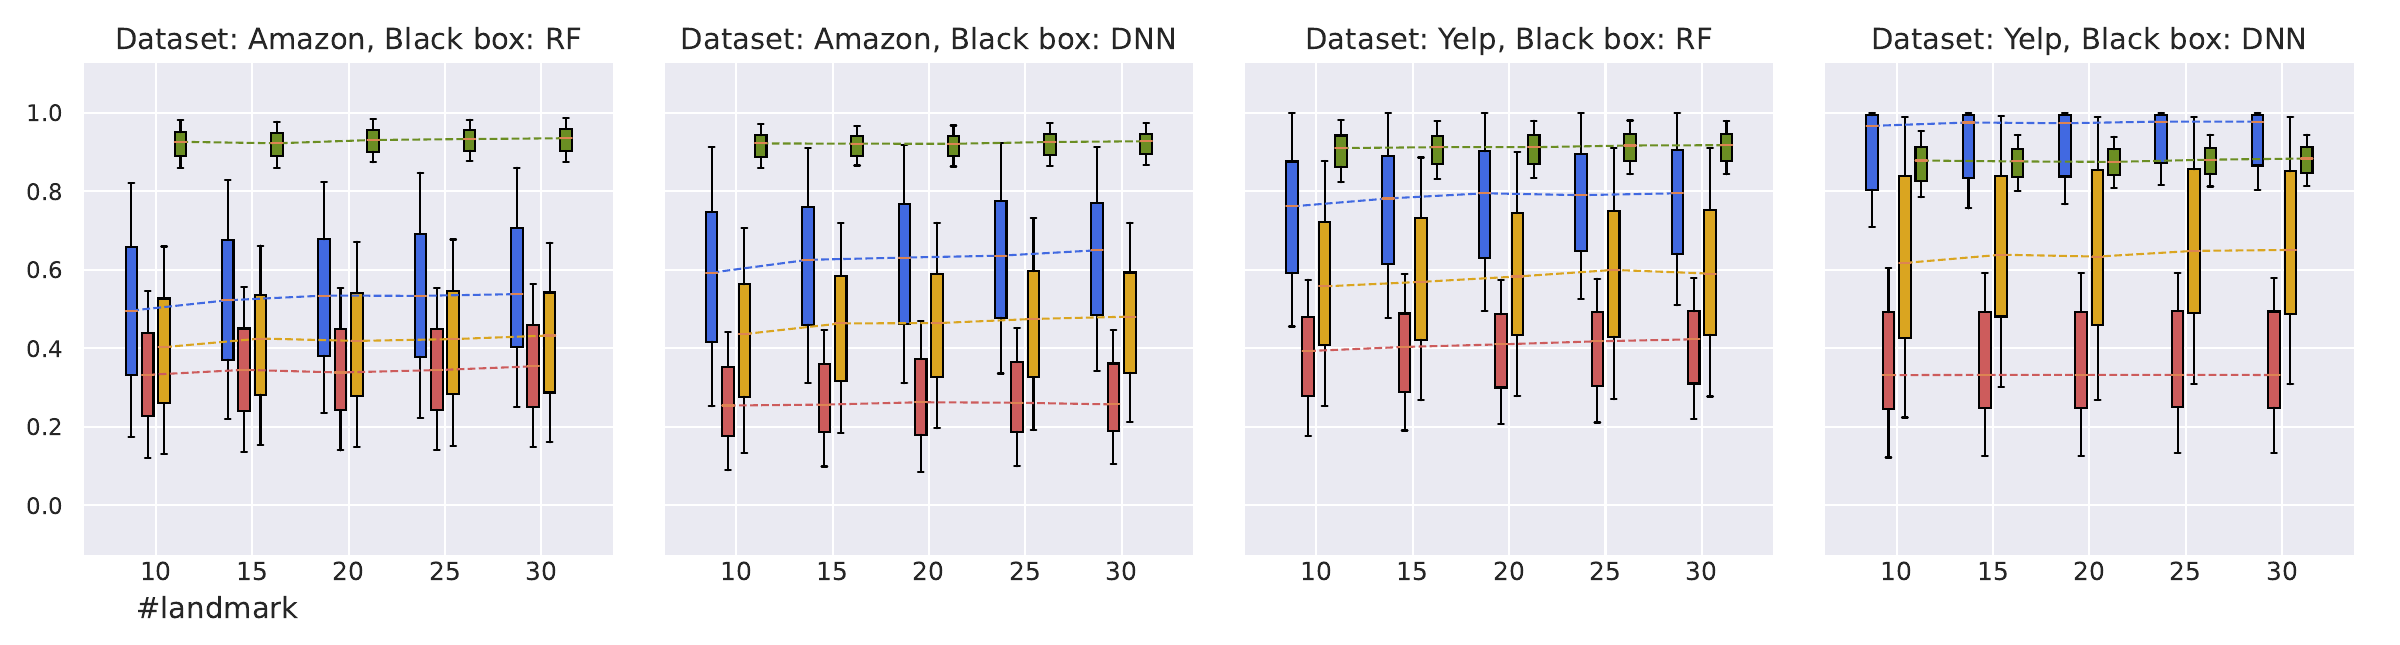}
        \vspace*{-8mm}
        \caption{Sensitivity to the number of landmarks, the interpolation step is fixed to 10.}
        \label{fig:xproaLm}
    \end{subfigure}
    \vspace*{-8mm}
    \caption{Sensitivity to hyperparameters of the neighborhood approximation in \gbased }
    \label{fig:xproa_sen}
\end{figure*}

\begin{figure*}
    \centering
    \begin{subfigure}[b]{1.\textwidth}
        \centering
        \includegraphics[width=\textwidth]{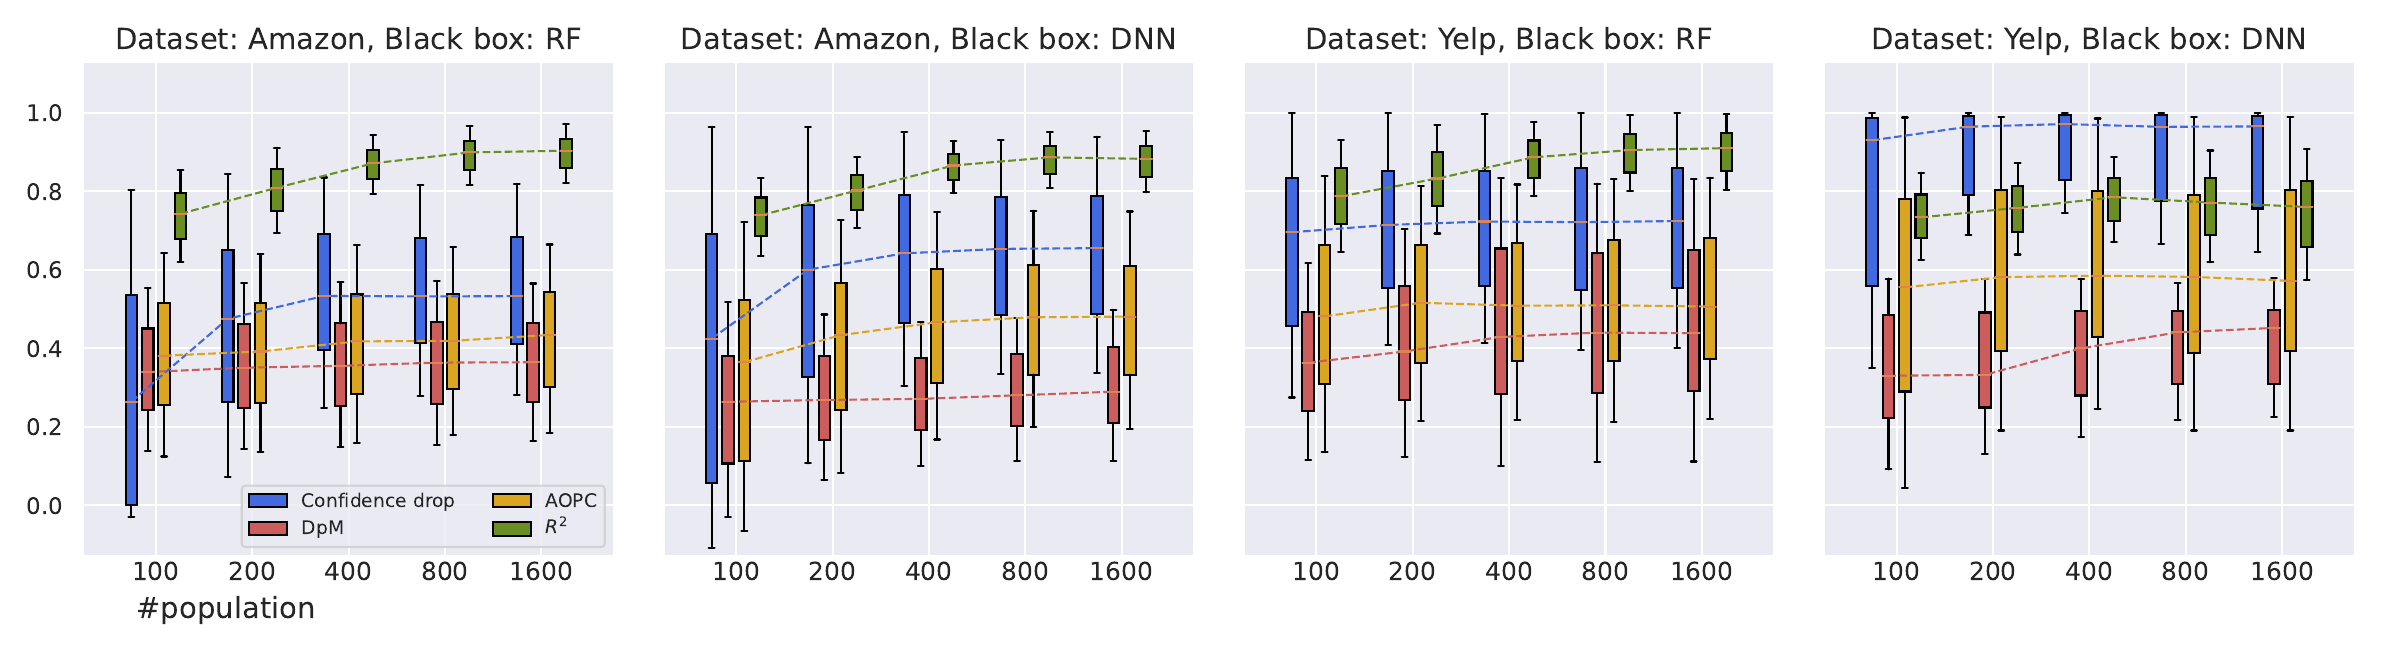}
        \vspace*{-8mm}
        \caption{Sensitivity to the neighborhood size, the number of prototypes is fixed to 80.}
        \label{fig:xprobPopu}
    \end{subfigure}
    \vspace*{3mm}
    \begin{subfigure}[b]{1.\textwidth}
        \centering
        \includegraphics[width=\textwidth]{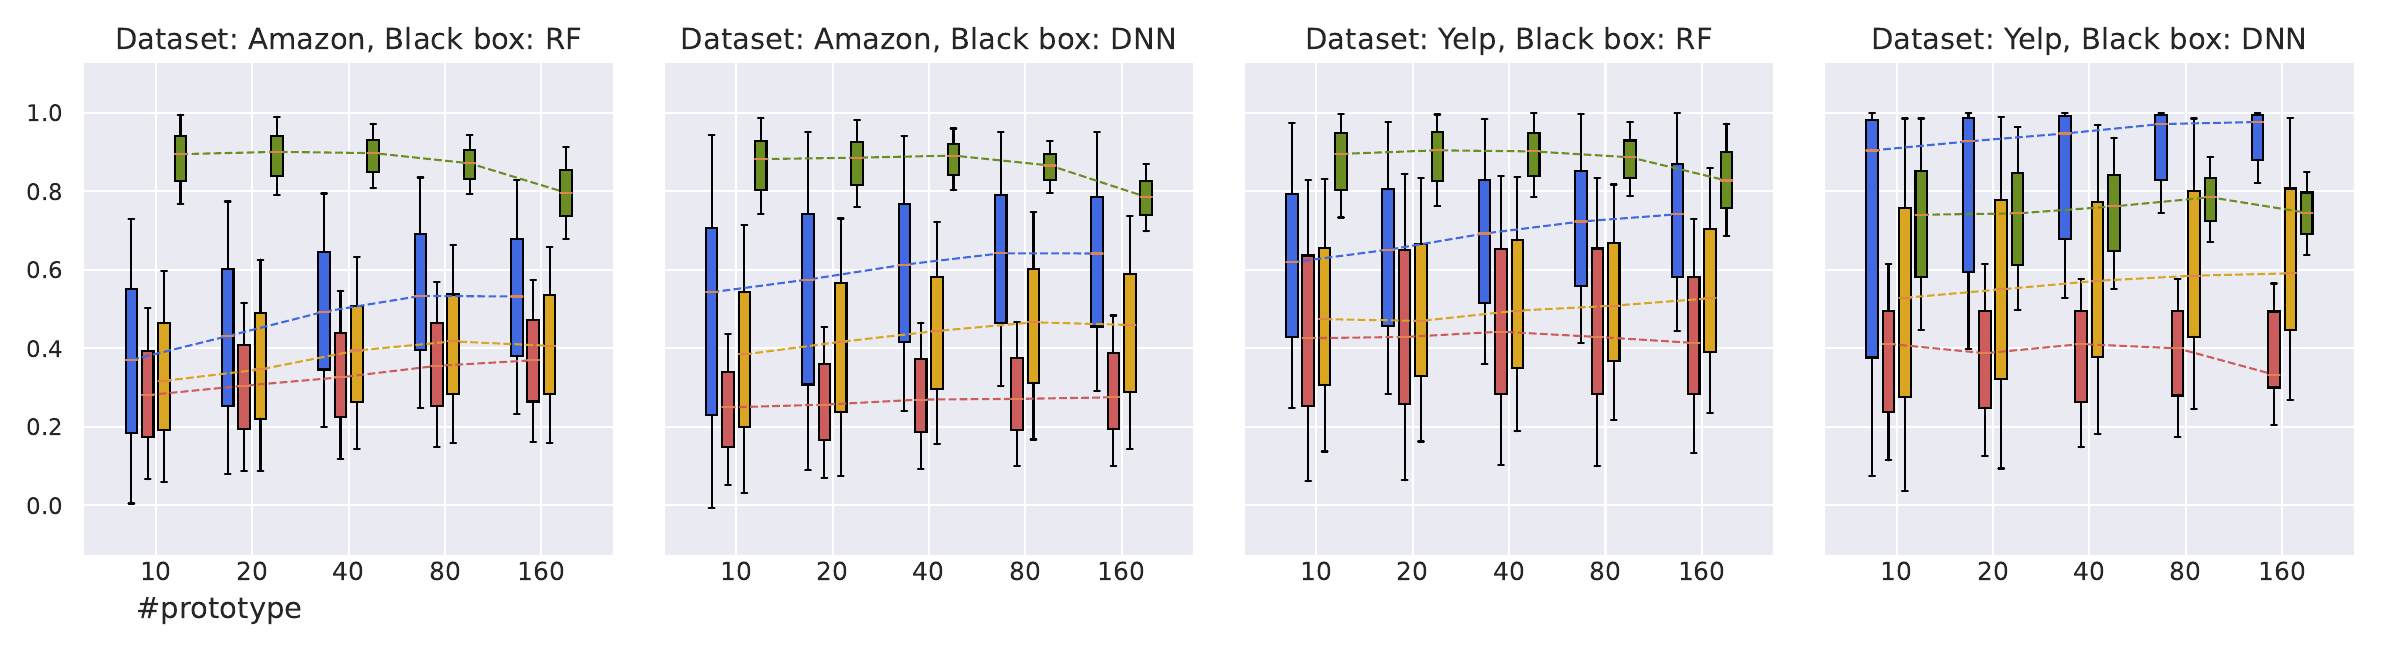}
        \vspace*{-8mm}
        \caption{Sensitivity to the number of prototypes, the population is fixed to 400.}
        \label{fig:xprobLm}
    \end{subfigure}
    \vspace*{-8mm}
    \caption{Sensitivity to hyperparameters of the neighborhood approximation in \pbased }
    \label{fig:xprob_sen}
\end{figure*}

Although we applied the same hyperparameter setting throughout the experiments, the plots in Fig.~\ref{fig:xproa_sen} and Fig.~\ref{fig:xprob_sen} show that the optimal choices are not identical under different settings.
In reality, the best hyperparameter choice depends on the data distribution and the decision boundary of the explaining target.
% It would be time-consuming if the goal is determining optimal neighborhoods.

\section{Dependencies on external resources} \label{apx:dependencies}
We follow the same experimental settings described in Section~\ref{sec:dependency} and report in Tables~\ref{tbl:appendix_dependency_gen} and~\ref{tbl:appendix_dependency_corpus} the dependencies of \gbased{} and \pbased{} on external resources while explaining different models.
In general, the results match the ones reported previously.
The quality of explanations improves consistently with the enrichment of external knowledge.
The performance tends to remain stable when the resources become sufficiently informative.
However, the definition of external resource sufficiency is shown to be case-specific.
For example, there is potential for better performances of \gbased{}~in explaining decisions from the \textit{yelp RF} and \textit{yelp LSTM} classifiers. 
The same holds for \pbased{}~tested on the \textit{yelp LSTM} classifier.

Again, the differences in performance between the utilization of the two kinds of generators highlight themselves. 
The results of the control group suggest that the fulfillment of the reconstruction ability and the locality-preserving property has higher priority than the enhancement of the generator capacity.

\begin{table*}[tbp]
\caption{Dependency of \gbased{} on generative models}
\label{tbl:appendix_dependency_gen}
\centering
\begin{tabular}{|cc|c|cc||c|cc|cc|} 
\hline
% Corpus size & C. D. & \makecell{DpM} & AOPC\Tstrut\\
\multicolumn{2}{|c|}{\multirow{2}{*}{\textbf{Generator}}} & \multirow{2}{*}{{$\mathcal{L}_{rec}$}}
& \multicolumn{2}{c||}{\textbf{Amazon BERT}} &
\multirow{2}{*}{{$\mathcal{L}_{rec}$}} & \multicolumn{2}{c|}{\textbf{Yelp BERT}} & \multicolumn{2}{c|}{\textbf{Yelp LSTM}}\Tstrut\\
% \cline{1-11}
% \cline{4-5} \cline{7-10}
& & & Confidence drop & AOPC & & Confidence drop & AOPC & Confidence drop & AOPC\Tstrut\\
\hline

\multirow{4}{*}{DAAE} & 32 & 11.77 
& 0.442 ± 0.395 & 0.379 ± 0.356
% ------------------ YELP
& 9.40
& 0.654 ± 0.457 & 0.537 ± 0.409
& 0.750 ± 0.373 & 0.562 ± 0.326\Tstrut\\

& 64 & 5.47 
& 0.539 ± 0.382 & 0.462 ± 0.342
% ------------------ YELP
& 4.65
& 0.738 ± 0.423 & 0.615 ± 0.388
& 0.817 ± 0.311 & 0.608 ± 0.286\\

& 96 & 4.18 
& 0.559 ± 0.359 & 0.478 ± 0.332
% ------------------ YELP
& 3.13
& 0.753 ± 0.410 & 0.617 ± 0.375
& 0.816 ± 0.307 & 0.609 ± 0.280\\

& 128 & 3.93 
& \textbf{0.583 ± 0.369} & \textbf{0.484 ± 0.329}
% ------------------ YELP
& 2.79
& \textbf{0.770 ± 0.401} & \textbf{0.629 ± 0.366}
& \textbf{0.827 ± 0.299} & \textbf{0.623 ± 0.278}\\

\hline
\hline

\multirow{4}{*}{VAE} & 32 & 25.23 
& 0.307 ± 0.399 & 0.265 ± 0.355
% ------------------ YELP
& 19.75
& \underline{0.531 ± 0.488} & \underline{0.444 ± 0.428}
& \underline{0.577 ± 0.449} & \underline{0.431 ± 0.358}\Tstrut\\

& 64 & 25.72 
& 0.287 ± 0.391 & 0.251 ± 0.345
% ------------------ YELP
& 21.57
& 0.475 ± 0.486 & 0.395 ± 0.427
& 0.461 ± 0.452 & 0.343 ± 0.350\\

& 96 & 27.00 
& \underline{0.315 ± 0.394} & \underline{0.267 ± 0.351}
% ------------------ YELP
& 21.98
& 0.482 ± 0.487 & 0.411 ± 0.433
& 0.539 ± 0.444 & 0.416 ± 0.357\\

& 128 & 27.75 
& 0.306 ± 0.403 & 0.247 ± 0.361
% ------------------ YELP
& 21.94
& 0.505 ± 0.487 & 0.429 ± 0.435
& 0.516 ± 0.445 & 0.393 ± 0.350\\
\hline
% 2k  & 0.477 & 0.317 & 0.392 
%     & 0.638 & 0.383 & 0.501 
%     & 0.790 & 0.340 & 0.568\Tstrut\\
    
% 5k  & 0.494 & 0.320 & 0.394 
%     & 0.665 & 0.386 & 0.513 
%     & 0.795 & 0.347 & 0.567\\
    
% 10k & 0.511 & 0.325 & \textbf{0.405}
% & 0.659 & 0.385 & 0.507
% & 0.800 & 0.351 & 0.576\\

% 20k & 0.515 & 0.324 & 0.404 
% & 0.673 & \textbf{0.387} & 0.516 
% & 0.822 & \textbf{0.359} & \textbf{0.589}\\

% 40k & \textbf{0.516} & 0.329 & 0.403 
% & \textbf{0.685} & 0.386 & \textbf{0.524} 
% & 0.820 & 0.356 & 0.578\\

% 80k & 0.509 & \textbf{0.336} & 0.404 
% & 0.682 & 0.383 & 0.521 
% & \textbf{0.834} & 0.358 & 0.587\\
\hline
\end{tabular}
\end{table*}

\begin{table*}[tbp]
\caption{Dependency of \pbased{} on the size of the prototype corpus}
\label{tbl:appendix_dependency_corpus}
\centering
\begin{tabular}{|c|cc|cc|cc|} 
\hline
\multirow{2}{*}{\textbf{Corpus size}} & \multicolumn{2}{c|}{\textbf{Amazon BERT}} & \multicolumn{2}{c|}{\textbf{Yelp BERT}} & \multicolumn{2}{c|}{\textbf{Yelp LSTM}}\Tstrut\\
% \cline{1-11}
% \cline{2-10}
& Confidence drop & AOPC & Confidence drop & AOPC & Confidence drop & AOPC\Tstrut\\
\hline
2k  & 0.474 ± 0.352 & 0.391 ± 0.311
    & 0.702 ± 0.431 & 0.552 ± 0.383
    & 0.784 ± 0.321 & 0.622 ± 0.303\Tstrut\\
    
5k  & 0.533 ± 0.350 & 0.444 ± 0.313
    & 0.739 ± 0.413 & 0.589 ± 0.376
    & 0.806 ± 0.311 & 0.644 ± 0.295\\
    
10k & 0.569 ± 0.345 & 0.481 ± 0.316
& 0.745 ± 0.413 & 0.591 ± 0.373
& 0.806 ± 0.307 & 0.640 ± 0.297\\

20k & 0.584 ± 0.345 & 0.482 ± 0.311
& 0.760 ± 0.405 & 0.609 ± 0.372
& 0.822 ± 0.296 & 0.658 ± 0.288\\

40k & 0.592 ± 0.334 & 0.491 ± 0.309
& 0.769 ± 0.399 & 0.616 ± 0.366
& 0.836 ± 0.279 & 0.670 ± 0.278\\

80k & \textbf{0.599 ± 0.334} & \textbf{0.493 ± 0.306}
& \textbf{0.780 ± 0.393} & \textbf{0.626 ± 0.369}
& \textbf{0.848 ± 0.268} & \textbf{0.666 ± 0.277}\\
\hline
\end{tabular}
\end{table*}
